# Supplementary material for: Bound and Conquer: Improving Triangulation by Enforcing Consistency
Source: arXiv:1804.10448 source file (2018-04-27)
Supplement: Supplementary file 1 [file x_appendix.tex]

\appendix
\section{Proof of the Theorems Presented in the Paper}
\subsection{Proof of the Inverse-Quadratic Dependence of the Accuracy of a Multi-Camera System on the Number of Cameras}
\label{appendix_proof_lobound}
	 A single camera with a resolution of $N\times N$ pixels partitions the world space into $N^2$ regions. Combined with the partitions of other cameras, this leads to a finite number of partitions. We split the expected reconstruction error over these partitions: 
	\begin{equation}
	\mathcal{E}=\frac{1}{\vol\Roi}\sum_{\mathcal{C}\in\mathcal{P}} \iiint_{\mathcal{C}} \left\| \hX-\X\right\|_{2}^2 d\X,
	\label{eq_av_loc_error_split}
	\end{equation}
	where the sum is taken over the set $\mathcal{P}$ of all partitions and $\vol\Roi$ represents the volume of the region of interest (ROI). 
	%where $\mathcal{T}$ is the set of all valid feature trajectories and we have defined $\boldsymbol{\hat{s}_q}\coloneqq\mathcal{S}_{\Phi,\Lambda}(Q_\Lambda(\mathcal{P}_{\Phi}(\boldsymbol{s})))$ to emphasise that it is fixed given the feature trajectory $\boldsymbol{q}$.
	
	The localisation error over each partition, i.e. the integral $\iiint_{\mathcal{C}} \left\| \hX-\X\right\|_{2}^2 d\X$, depends on both its size and shape. Among all partitions with the same volume, the value of this integral would be minimised if the shape was a sphere and the estimate, $\hX$, was at the centre of that sphere:
	\begin{equation}
	\iiint_{\mathcal{C}} \left\| \hX-\X\right\|_{2}^2 d\X \geq \iiint_{H_r} \left\| \boldsymbol{c}-\X\right\|_{2}^2 d\X,
	\label{eq_prlb}
	\end{equation}
	where $H_r$ is a sphere with centre $\boldsymbol{c}$ and radius $r=\sqrt[3]{3\vol{\mathcal{C}}/(4\pi)}$. 
	
	By converting to polar coordinates, we obtain
	\begin{align*}
	\iiint_{H_r} \left\| \boldsymbol{c}-\X\right\|_{2}^2 d\X&=\int_0^{2\pi} \int_0^{\pi} \int_0^r t^2 t^2 dt d\theta\\
	&= \frac{2\pi^2}{5} r^5= \frac{2\pi^2}{5} \sqrt[3]{\frac{3}{4\pi}} \vol{\mathcal{C}}^\frac{5}{3},\label{eq_rhs_int}
	\end{align*}
	which when combined with \eqref{eq_av_loc_error_split} and \eqref{eq_prlb} yields
	\begin{align}
	\mathcal{E}&=\frac{1}{\vol\Roi}\sum \iiint_{\mathcal{C}} \left\| \hX-\X\right\|_{2}^2 d\X\\
	&> \frac{1}{\vol\Roi}\sum_{\mathcal{C}\in\mathcal{P}} \frac{2\pi^2}{5} \sqrt[3]{\frac{3}{4\pi}} \vol{\mathcal{C}}^\frac{5}{3}.
	\end{align}
	Hence, we have a lower bound for $\mathcal{E}$ in terms of the size $\vol{\mathcal{C}}$ and the total number $\#\mathcal{P}$ of partitions. This lower-bound would be minimised if the available volume, $\vol\Roi$, was split equally among the regions:
	\begin{align}
	\mathcal{E}&> K\frac{1}{\vol\Roi}\sum  \left(\frac{\vol\Roi}{\#\mathcal{P}}\right)^\frac{5}{3}
	=K\left(\frac{\vol\Roi}{\#\mathcal{P}}\right)^\frac{2}{3},	
	\label{eq_lb_av_err_num_of_regions}
	\end{align}
	where $K=\frac{2\pi^2}{5} \sqrt[3]{\frac{3}{4\pi}}$.

	%The total number of partitions induced by a multi-camera system is given by the cardinality of the set $\mathcal{P}$, denoted $\#\mathcal{P}$. 

	Finally, knowing that the volume $\vol\Roi$ of the region of interest is fixed, the last remaining step in inferring our lower bound is to consider how the number of regions $\#\mathcal{P}$ grows as we add more cameras to the system, or to bound the total number of partitions $\#\mathcal{P}$.

	To do so, we first consider how many regions can be created from $L$ planes in $\mathbb{R}^3$. In computational geometry, this quantity that we want to bound is known as the number of cells in an arrangement of hyperplanes (see for example \cite{Berg2008Compgeometry}). It can be shown that, with $L$ planes, the 3-D space $\mathbb{R}^3$ is partitioned into at most $k$ regions and $k$ grows cubically with $L$, i.e. $k=\mathcal{O}(L^3)$.   
	
	In our case partitions created by the boundaries of the pixels in a multi-camera system, we can see that each camera in a multi-camera system partitions the space with $(N+1)^2$ planes intersected by rays starting from the camera centre and passing through pixel boundaries~\footnote{In the case of orthogonal projection, rays do not originate from the centre of the camera, but their cardinality and hence the rest of the proof remain unchanged.}. In total, there are $M(N+1)^2$ such rays and thus we can conclude that the number of regions $\#\mathcal{P}$ satisfies
	\begin{equation}
	\#\mathcal{P} =  \mathcal{O}({M^3N^6}).
	\label{eq_ub_num_regions}
	\end{equation}
	Substituting \eqref{eq_ub_num_regions} into \eqref{eq_lb_av_err_num_of_regions} gives
	\begin{equation*}
	\mathcal{E} =\Omega (\frac{\vol\Roi}{M^2N^4}),
	\end{equation*}
	which proves that $\mathcal{E}=\Omega\left(\frac{1}{M^2}\right)$ for fixed $N$ and $\mathcal{R}$, hence the fact that best possible decay rate for a geometric reconstruction algorithm is quadratic.
