# Supplementary material for: Bound and Conquer: Improving Triangulation by Enforcing Consistency
Source: arXiv:1804.10448 source file (2018-04-27)
Supplement: Supplementary file 2 [file 8_appendix.tex]

%\appendix
%\subsection*{Maximum-likelihood estimator assuming a Gaussian noise model}
%\begin{lemma}
%	Minimising the $\ell_2$-norm of the residual vector is the maximum-likelihood estimator assuming each image point is perturbed with independently and identically distributed (i.i.d.) zero-mean Gaussian noise.
%	\label{th_l2_gauss}
%\end{lemma}
%
%\begin{proof}
%	Assume we add i.i.d. noise to each image point, yielding
%	\begin{equation}
%	\x_i=\cP_i\X+\epsilon_i,
%	\end{equation}
%	where $\epsilon_i\sim \mathcal{N}(0,\sigma)$ and $\X$ is the latent variable we aim to estimate. Then,
%	\begin{equation}
%	\x_i\sim \mathcal{N}(\cP_i\X,\sigma).
%	\end{equation}
%	
%	The maximum likelihood estimator of $\X$ is thus
%	\begin{equation}
%	\hX=\argmax_\bX \prod_i K\exp\left(-\frac{|| \x_i - \cP_i\bX||_{p'}^2}{2\sigma^2}\right)
%	\end{equation}
%	where $K$ is a normalising constant. By taking the natural logarithm it is easy to show that
%	\begin{equation}
%	\hX=\argmin_\bX \sum || \x_i - \cP_i\bX ||_{p'}^2,
%	\label{eq_gauss_mle}
%	\end{equation} 
%	which proves the lemma.
%\end{proof}

%\subsection*{Maximum-likelihood estimator assuming a uniform noise model}
%\begin{lemma}
%	Minimising the $\lf$ norm to solve a geometric reconstruction problem is equivalent to solving the problem using maximum-likelihood estimation assuming a uniform noise model. \label{th_linf_unif}
%\end{lemma}
%
%\begin{proof}
%	Assume the distribution of the noise follows the following distribution:
%	\begin{equation}
%	f(\epsilon)=K\exp\left(- \frac{|| \epsilon||_{p'}^p}{\delta^p} \right),
%	\label{eq_lp}
%	\end{equation}
%	with $K$ a normalising constant and $p$ and $p'$ being the residual-space norm and image-space norm, respectively. Using this model and with the same arguments as in the $\lii$-case, we can conclude that the maximum likelihood estimate is
%	\begin{equation}
%		\hX=\argmin_\bX \sum_i || \x_i - \cP_i\X||_{p'}^p.\label{eq_lp_mle}
%	\end{equation}
%	
%	Now, as $p\rightarrow\infty$, \eqref{eq_lp} converges to a symmetric uniform distribution, with width $\delta$~\cite{hartley2007optimal}. Moreover, \eqref{eq_lp_mle} converges to minimax problem given in \eqref{eq_lf}.
%\end{proof}
